# Supplementary material for: Better Together: Leveraging Unpaired Multimodal Data for Stronger Unimodal Models
Source: arXiv:2510.08492 source file (2025-10-09)
Supplement: Supplementary file 1 [file audio_image_fewshot_clip_rn50.tex]

\begin{table}[!htb]
  \centering
\begin{minipage}[t]{1.\linewidth}
\centering
\caption{\textbf{Linear evaluation of frozen features on audio classification on audio-visual benchmarks}. We compare our proposed approach with the audio-only baseline and show that incorporating unpaired image and text data can significantly improve audio classification under few-shot scenarios (CLIP RN50 backbone)\todo{Correct numbers in braces.}}
\resizebox{.8\textwidth}{!}{%

  \begin{tabular}{ll|lll}
    \toprule
    Dataset          & Method                 & \multicolumn{3}{c}{Audio Classification} \\
    \cmidrule(lr){3-5}
                     &                        & 1-shot & 2-shot & 4-shot \\
    \midrule
    \multirow{3}{*}{ImageNet-ESC-19}
                     & Audio-Only      & 28.78   & 39.85   & 52.24   \\
                     % & Audio + Image      & \textbf{34.15} & 43.80 & 55.57 \\
                     % & Audio + Text      & 32.94 & \textbf{44.41} & \textbf{57.61} \\
                     & Audio + Image          & {34.59}  \increase{44.60}
                                               & 44.13  \increase{3.34}
                                               & 50.00  \increase{1.52} \\
                     & Audio + Text           & 35.47  \increase{3.39}
                                               & {52.19}  \increase{3.95}
                                               & {52.90}  \increase{3.56} \\
                     
    \midrule
    \multirow{3}{*}{ImageNet-ESC-27}
                     & Audio-Only & 25.65 & 35.99 & 44.79     \\
                      & Audio + Image          \\
                     & Audio + Text     \\
    \bottomrule
  \end{tabular}
  }
  \end{minipage}
  \label{tab:audio-image-fewshot-clip-rn50}
\end{table}

\begin{table}[!htb]
  \centering
\begin{minipage}[t]{1.\linewidth}
\centering
\caption{\textbf{Linear evaluation of frozen features on image classification on audio-visual benchmarks}. We compare our proposed approach with the audio-only baseline and show that incorporating unpaired image and text data can significantly improve audio classification under few-shot scenarios (CLIP RN50 backbone)\todo{Correct numbers in braces.}}
\resizebox{.8\textwidth}{!}{%

  \begin{tabular}{ll|lll}
    \toprule
    Dataset          & Method                 & \multicolumn{3}{c}{Image Classification} \\
    \cmidrule(lr){3-5}
                     &                        & 1-shot & 2-shot & 4-shot \\
    \midrule
    \multirow{3}{*}{ImageNet-ESC-19}
                     & Image-Only      & 60.28   & 74.10   & 78.70   \\
                     % & Audio + Image      & \textbf{34.15} & 43.80 & 55.57 \\
                     % & Audio + Text      & 32.94 & \textbf{44.41} & \textbf{57.61} \\
                     & Image + Audio        & {64.35}  \increase{44.60}
                                               & 78.73  \increase{3.34}
                                               & 81.64  \increase{1.52} \\
                     & Image + Text   \\
                     
    \midrule
    \multirow{3}{*}{ImageNet-ESC-27}
                     & Image-Only & 51.75 & 70.76 & 75.16\\
                      & Image + Audio          \\
                     & Image + Text   \\
    \bottomrule
  \end{tabular}
  }
  \end{minipage}
  \label{tab:image-audio-fewshot-clip-rn50}
\end{table}
